# Supplementary material for: Neural Packing: from Visual Sensing to Reinforcement Learning
Source: arXiv:2311.09233 source file (2023-10-17)
Supplement: Supplementary file 1 [file 6-appendix.tex]

\newpage

\section{Appendix}

\subsection{Object detection}

	For the object extraction, as shown in Figure~\ref{fig:detect}, we first use the Mask RCNN network~\cite{he2017mask} to detect the objects, which takes the RGBD image as input and outputs the instance mask of each observed box. For each masked object, we obtain its point cloud using associated depth information and further estimate its dimensions and 6D pose using the cuboid fitting algorithm~\cite{jiang2013linear}. 
	
\subsection{Object encoder}

Figure~\ref{fig:shape_enc} shows the structure of the object encoder. 
%Taking each box state data $B_i$ as input, we apply an MLP layer for the box shape feature, which is then further concatenated with the precedence feature, resulting in $s_i$ as the embedded object feature of $B_i$. 
%In more details, for a given input $P_i$, where $P_{ik}\in \{0,1\}^{2}$ is the block relation between box state $i$ and box $k$. We apply an MLP layer to encode each $\{P_{ik}\}_{k=1,\dots,n}$ to feature $\{p_{ik}\}_{k=1,\dots,n}$, and then the features are passed to a transformer encoder to get the precedence feature, where all the features $\{p_{ik}\}$ are used as the key matrix $k$ and value matrix $v$ of attention module, and the feature $p_{ii}$ is the query matrix $q$.
\rh{Taking each box state $B_i = \{b_i, P_i\}$ as input, the shape feature and precedence feature are extracted separately and then concatenated to obtain the final object feature  $s_i$.
	In more detail, we apply an MLP layer to $b_i$ to extract the shape feature, while using a more complicated Transformer encoder to extract the precedence feature from $P_i$, where $P_i = \{P_{ij}\}_{j=1}^{n}$ with $P_{ij} \in \{0,1\}^{2}$ indicating the block relation between box state $B_i$ and box $j$. 
	Specifically, we first apply another MLP layer to encode each $P_{ij}$ to feature $p_{ij}$ and then pass all those features to a Transformer encoder to get the precedence feature,  where all the features $\{p_{ij}\}$ are used as the key matrix $k$ and value matrix $v$ of attention module, and the feature $p_{ii}$ is the query matrix $q$ for $B_i$.}
%the shape feature and precedence feature are encoded $$}
\mlc{try to simplify the above sentence.}
For simplicity, we only show the indexes of objects with corresponding precedence edges pointing to the given object in the left of Figure~\ref{fig:network}, but show the one-hot representation for the example box $b_i$ in Figure~\ref{fig:shape_enc}.

\begin{figure}[!t]
    \centering
    \includegraphics[width=0.49\textwidth]{images/object_detection.pdf}
\caption{Object extraction. Given the RGBD image captured from the source objects, our method first uses the Mask RCNN network~\cite{he2017mask} to detect the objects, and then uses the cuboid fitting algorithm~\cite{jiang2013linear} to estimate the size and 6D pose of each detected object.}
\label{fig:detect}
\end{figure}

\begin{figure}[!t]
    \centering
    \includegraphics[width=0.49\textwidth]{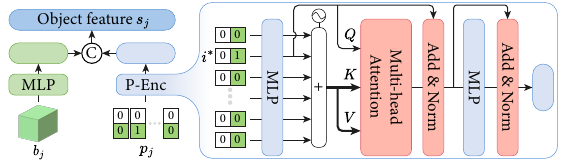}
\caption{The detailed structure of the object encoder as part of the Source Encoder in Figure~\ref{fig:network}.}
\label{fig:shape_enc}
\end{figure}

\subsection{Experiment}

\begin{table}[!t]%
	\caption{Performance of TAP-Net++ trained on data with different quantization levels, but all tested on data with unit length $u=1$.
	For each test shape, we represent it using either the \emph{approximate} size with the training quantization level $u$ or the \emph{actual} size with $u=1$ to get two sets of results. 
	\mlc{it is a bit confusing here to explain approximate vs actual.  Can we test a matrix of performance between Du and Tu? Du=20 vs Tu=20, 10, 5, 1;  Du=20 vs Tu=10, 5, 1; Du=5 vs Tu=5, 1.}}
	\label{tab:diff_prec}
	\begin{minipage}{\columnwidth}
		\begin{center}
			\begin{tabular}{l||l|l|l|l}
				\hline
				\textbf{Training $u$} & 20 & 10 & 5 & 1 \\ \hline
				\textbf{Approximate} & 0.522 & 0.588 & 0.623 & 0.648 \\ \hline
				\textbf{Actual} & 0.638 & 0.648 & 0.647 & 0.648 \\ \hline
			\end{tabular}
			
		\end{center}
	\end{minipage}
\end{table}%

In the second experiment, we test whether our network trained on data with one unit length can generalize well to another unit length.  
In particular, we are interested in whether the network trained using inaccurate measurements (large $u$ value) can handle more accurate measurements (small $u$ value).
%Furthermore, we also test our network trained on data with different unit lengths, but test on data with the finest unit length 1.
Table~\ref{tab:diff_prec} shows the performance of TAP-Net++ trained on $D_u$ with various $u$ but all tested on $T_1$.
For each shape in $T_1$, we represent it using either the \textbf{approximate} size with the training quantization level $u$ or the \textbf{actual} size with $u=1$ for testing.  \mlc{see my comments in caption.}
Figure~\ref{fig:approximate_test} shows the packing results when the packing strategy is optimized using \textbf{approximate} sizes with different $u$. 
With the increase of $u$, the approximation of the box becomes more and more inaccurate, which leads to large gaps and empty spaces in the final packing results.

As shown in the \textbf{Actual} column in Table~\ref{tab:approximate_test}, we can see that our network trained on data with different unit lengths can get comparable results to the network trained directly on data with the finest unit length $u=1$, and get far more compact results than directly representing the test data using the training quantization level shown in the  \textbf{Approximate} column. 
This indicates the generality of our method to handle data with different measurement accuracy when captured using different devices.

%we can train our network with boxes on various precision, when we test boxes on different precision, there are two methods to using our network: The first method is using the approximate box size on training precision as network input to compute all the packing positions, then we pack the actual box size at their corresponding positions. The second method is using actual box sizes as input directly. Table~\ref{tab:approximate_test} shows the performance of our network under different testing methods, we train the network with different precision and test the data with precision $1$, the method using approximate size causes a lot of space wasted, while the method using actual size directly gets more compact packing. This result also indicates the generality of our network, so in the rest of the experiments, we use the second method to test the network on different precision.
 
\begin{figure}[!t]
    \centering
    \includegraphics[width=0.49\textwidth]{images/approximate_test.pdf}
\caption{\rh{Packing results of networks training on with different quantization levels when tested on the same set of shapes but with size approximated using the corresponding quantization level.}}
\label{fig:approximate_test}
\end{figure}

%\subsection{Baseline Comparisons}
